# Supplementary material for: Not So Fast: Understanding and Mitigating Negative Impacts of Compiler Optimizations on Code Reuse Gadget Sets
Source: arXiv:2005.08363 source file (2021-09-29)
Supplement: Supplementary file 1 [file A_appendix.tex]

\section{Appendices}

\subsection{Single Optimization Variants Analyzed}
\label{app:single_optimizations}

Table \ref{tab:gcc_single} contains the single optimization variants that were generated using the \verb|GCC| compiler for this study. Table \ref{tab:clang_single} contains the single optimization variants that were generated using the \verb|Clang|. In both tables, the column identifier indicates the baseline optimization that the single optimization variant was compared against using GSA. Although single-optimization variants were built for all benchmark programs for our fine-grained analysis in Section \ref{section:fine_grained}, the majority of single-optimization variants were derived from our common Linux benchmarks.

\begin{table*}
\centering
    \footnotesize
    \caption{GCC Single Optimization Variants Studied}
    \label{tab:gcc_single}
    {\rowcolors{2}{lightgray!50}{white}
\begin{tabular}{|l|l|l|}
    \hline
    \multicolumn{1}{|c|}{\textbf{O0} (included in O1)} & \multicolumn{1}{c|}{\textbf{O1}(included in O2)} & \multicolumn{1}{c|}{\textbf{O2}(included in O3)} \\
    \hline
    (1) tree-sink & (35) partial-inlining & (73) peel-loops\\
    (2) ipa-profile & (36) ipa-icf & (74) tree-loop-vectorize\\
    (3) tree-bit-ccp & (37) indirect-inlining & (75) inline-functions\\
    (4) branch-count-reg & (38) tree-tail-merge & (76) predictive-commoning\\
    (5) forward-propagate & (39) reorder-functions & (77) tree-slp-vectorize\\
    (6) compare-elim & (40) ipa-ra & (78) split-paths\\
    (7) ssa-phiopt & (41) isolate-erroneous-paths-dereference & (79) tree-partial-pre\\
    (8) tree-ch & (42) ipa-cp & (80) tree-loop-distribute-patterns\\
    (9) cprop-registers & (43) reorder-blocks-and-partition & (81) unswitch-loops\\
    (10) tree-dse & (44) caller-saves & (82) ipa-cp-clone\\
    (11) ipa-reference & (45) expensive-optimizations & (83) split-loops\\
    (12) tree-sra & (46) ipa-icf-variables & (84) gcse-after-reload\\
    (13) tree-builtin-call-dce & (47) optimize-strlen & \\
    (14) tree-fre & (48) crossjumping & \\
    (15) tree-coalesce-vars & (49) ipa-vrp & \\
    (16) split-wide-types & (50) thread-jumps & \\
    (17) tree-ccp & (51) ipa-icf-functions & \\
    (18) tree-dce & (52) gcse & \\
    (19) reorder-blocks & (53) code-hoisting & \\
    (20) tree-dominator-opts & (54) strict-overflow & \\
    (21) tree-pta & (55) devirtualize-speculatively & \\
    (22) inline-functions-called-once & (56) devirtualize & \\
    (23) tree-ter & (57) cse-follow-jumps & \\
    (24) guess-branch-probability & (58) ira-remat & \\
    (25) move-loop-invariants & (59) rerun-cse-after-loop & \\
    (26) ipa-pure-const & (60) tree-switch-conversion & \\
    (27) defer-pop & (61) hoist-adjacent-loads & \\
    (28) tree-slsr & (62) store-merging & \\
    (29) omit-frame-pointer & (63) align-labels & \\
    (30) shrink-wrap & (64) schedule-insns2 & \\
    (31) tree-copy-prop & (65) ipa-sra & \\
    (32) if-conversion & (66) peephole2 & \\
    (33) combine-stack-adjustments & (67) tree-vrp & \\
    (34) if-conversion & (68) ipa-bit-cp & \\
     & (69) optimize-sibling-calls & \\
     & (70) inline-small-functions & \\
     & (71) tree-pre & \\
     & (72) strict-aliasing & \\
    \hline
\end{tabular}
}
\end{table*}

\begin{table*}
\centering
    \footnotesize
    \caption{Clang Single Optimization Variants Studied}
    \label{tab:clang_single}
    {\rowcolors{2}{lightgray!50}{white}
\begin{tabular}{|l|l|l|l|}
    \hline
    \multicolumn{2}{|c|}{\textbf{O0} (included in O1)} & \multicolumn{1}{c|}{\textbf{O1} (included in O2)} & \multicolumn{1}{c|}{\textbf{O2} (included in O3)} \\
    \hline
    (1) loop-deletion & (21) bdce & (41) mldst-motion & (47) callsite-splitting\\
    (2) loop-distribute & (22) loop-simplify & (42) gvn & (48) aggressive-instcombine\\
    (3) sroa & (23) instcombine & (43) slp-vectorizer & (49) argpromotion\\
    (4) adce & (24) jump-threading & (44) constmerge & \\
    (5) memcpyopt & (25) simplifycfg & (45) inline & \\
    (6) deadargelim & (26) div-rem-pairs & (46) elim-avail-extern & \\
    (7) correlated-propagation & (27) libcalls-shrinkwrap &  & \\
    (8) loop-rotate & (28) globaldce &  & \\
    (9) functionattrs & (29) dse &  & \\
    (10) loop-idiom & (30) loop-sink &  & \\
    (11) omit-frame-pointer & (31) loop-unroll &  & \\
    (12) lcssa & (32) loop-vectorize &  & \\
    (13) reassociate & (33) tailcallelim &  & \\
    (14) loop-load-elim & (34) alignment-from-assumptions &  & \\
    (15) speculative-execution & (35) licm &  & \\
    (16) loop-unswitch & (36) strip-dead-prototypes &  & \\
    (17) early-cse & (37) float2int &  & \\
    (18) indvars & (38) prune-eh &  & \\
    (19) sccp & (39) ipsccp &  & \\
    (20) globalopt & (40) called-value-propagation &  & \\
    \hline
\end{tabular}
}
\end{table*}
