# Supplementary material for: Not So Fast: Understanding and Mitigating Negative Impacts of Compiler Optimizations on Code Reuse Gadget Sets
Source: arXiv:2005.08363 source file (2021-09-29)
Supplement: Supplementary file 3 [file A_supp_code_size.tex]

{\rowcolors{3}{lightgray!50}{white}
\begin{tabular}{|l|c|c|c|c|c|c|}
    \hline
    & \multicolumn{3}{c|}{\textbf{GCC}} & \multicolumn{3}{c|}{\textbf{Clang}} \\
    \hline
    \textbf{Benchmark} & \textbf{O0} & \textbf{O3} & $\Delta$\textbf{O3} &  \textbf{O0} & \textbf{O3} & $\Delta$\textbf{O3}\\
    \hline
    Bftpd & & 314.6 & &  & 99.5 & \\
    libcUrl & & 485.2 &  &  & 455.6 & \\
    git &  & 19403.2 &  &  &  11195.0 &  \\
    gzip & & 433.4 &  &  &  108.6 & \\
    httpd & & 925.6 & &  &  842.3 & \\
    libsqlite & & 5024.5 &  &  & 6643.7 & \\
    401.bzip2 & & 110.6 &  &  & 98.5 &\\
    403.gcc & & 4750.1 &  &  & 4021.3 &  \\
    429.mcf &  & 26.9 &  & &  23.0 & \\
    433.milc & & 197.5 & &  & 176.9 &\\
    444.namd &  & 349.5 &  &  & 333.1 & \\
    445.gobmk &  &4746.6 &  &  & 4590.0 & \\
    456.hmmer &  &410.6 & &  & 376.5 & \\
    458.sjeng & & 205.1 & &  & 163.8 & \\
    462.libquantum & & 55.2 & &  & 59.7 & \\
    470.lbm & & 22.1 & &  & 22.2 & \\
    482.sphinx3 & & 278.8 & &  & 246.8 &\\
    \hline
\end{tabular}
}
