# Supplementary material for: Not So Fast: Understanding and Mitigating Negative Impacts of Compiler Optimizations on Code Reuse Gadget Sets
Source: arXiv:2005.08363 source file (2021-09-29)
Supplement: Supplementary file 5 [file A_clang_supp_speed.tex]

    % Data as percentage
\pgfplotstableread[row sep=\\,col sep=&]{
    bench & O0 & O3   \\
    Bftpd & 100 & 99.03\\
    libcUrl & 100 &  89.74\\
    git & 100 & 67.34\\
    gzip & 100 & 50.36\\
    httpd & 100 & 81.24\\
    libsqlite & 100 & 97.40\\
    401.bzip2 & 100 & 42.37 \\
    403.gcc & 100 &  52.02\\
    429.mcf & 100 &  54.92\\
    433.milc & 100 &  46.93\\
    444.namd & 100 &  33.51\\
    445.gobmk & 100 &  58.01\\
    456.hmmer & 100 &  21.92\\
    458.sjeng & 100 &  51.10\\
    462.libquantum & 100 &  40.13\\
    470.lbm & 100 &  61.40\\
    482.sphinx3 & 100 &  37.83\\
    }\suppclangperf
    

    % Raw data in seconds
    %Bftpd  & 3.122 \\
    %libcUrl & 22.41 \\
    %git  & 2.326\\
    %gzip  & 3.507\\
    %httpd  & 4.068\\
    %libsqlite  & 58.72\\
    %401.bzip2  & 478.8 \\
    %403.gcc  & 260.2 \\
    %429.mcf  & 308.7 \\
    %433.milc  & 495.6 \\
    %444.namd  & 330.4 \\
    %445.gobmk  & 452.1 \\
    %456.hmmer & 321.4 \\
    %458.sjeng  & 469.3 \\
    %462.libquantum  & 294.2 \\
    %470.lbm  & 257.7 \\
    %482.sphinx3  & 499.7 \\

\begin{figure}
\centering
\begin{tikzpicture}
\begin{axis}[
	xtick=data,
	x tick label style={rotate=45, anchor=east, font=\footnotesize},
	symbolic x coords={Bftpd, libcUrl, git, gzip, httpd, libsqlite, 401.bzip2, 403.gcc, 429.mcf, 433.milc,                    444.namd, 445.gobmk, 456.hmmer, 458.sjeng, 462.libquantum, 470.lbm, 482.sphinx3},
	ybar,
	width=\textwidth,
	height=.4\textwidth,
	bar width=.2cm,
	legend style={at={(0.8,1)}, anchor=north,legend columns=-1},
]
\addplot table[x=bench,y=O0]{\suppclangperf};
\addplot table[x=bench,y=O3]{\suppclangperf};
\legend{O0, O3}
\end{axis}
\end{tikzpicture}
\caption{Performance Comparison of Position-Independent O0 and O3 Clang Variants (\%)}\label{fig:suppclang_perf}
\end{figure}
