# Supplementary material for: Not So Fast: Understanding and Mitigating Negative Impacts of Compiler Optimizations on Code Reuse Gadget Sets
Source: arXiv:2005.08363 source file (2021-09-29)
Supplement: Supplementary file 6 [file A_gcc_supp_speed.tex]

\pgfplotstableread[row sep=\\,col sep=&]{
    bench & O0 & O3 \\
    Bftpd & 100 & 83.00  \\
    libcUrl & 100 & 99.05 \\
    git & 100 &  58.51\\
    gzip & 100 &  78.18\\
    httpd & 100 & 87.71\\
    libsqlite & 100 & 90.52 \\
    401.bzip2 & 100 & 46.92 \\
    403.gcc & 100 &  55.88\\
    429.mcf & 100 &  53.18\\
    433.milc & 100 & 60.10\\
    444.namd & 100 &  43.17\\
    445.gobmk & 100 & 58.11\\
    456.hmmer & 100 &  19.91\\
    458.sjeng & 100 &  55.41\\
    462.libquantum & 100 & 44.85  \\
    470.lbm & 100 &  64.25\\
    482.sphinx3 & 100 &  36.64\\
    }\suppgccperf
% O0 times
% 401.bzip2	1057.879
% 403.gcc	464.909
% 429.mcf	547.91
% 433.milc	810.957
% 444.namd	855.827667
% 445.gobmk	793.491667
% 453.povray	423.832333
% 456.hmmer	1647.650667
% 458.sjeng	915.469333
% 462.libquantum	687.104
% 470.lbm	491.973333
% 471.omnetpp	609.292
% 482.sphinx3	1357.718667
    %Data in Seconds
    %Bftpd  & 3.129\\
    %libcUrl  & 24.55\\
    %git  & 2.123 \\
    %gzip  & 3.788\\
    %httpd  & 4.316\\
    %libsqlite & 63.26\\
    %401.bzip2  & 496.4\\
    %403.gcc  & 259.8 \\
    %429.mcf  & 291.4 \\
    %433.milc  & 487.4\\
    %444.namd  & 369.5 \\
    %445.gobmk  & 461.1\\
    %456.hmmer  & 328.1 \\
    %458.sjeng  & 507.3 \\
    %462.libquantum  & 308.2 \\
    %470.lbm  & 316.1 \\
    %482.sphinx3 & 497.5 \\
    
\begin{figure}
\centering
\begin{tikzpicture}
\begin{axis}[
	xtick=data,
	x tick label style={rotate=45, anchor=east, font=\footnotesize},
	symbolic x coords={Bftpd, libcUrl, git, gzip, httpd, libsqlite, 401.bzip2, 403.gcc, 429.mcf, 433.milc,                    444.namd, 445.gobmk, 456.hmmer, 458.sjeng, 462.libquantum, 470.lbm, 482.sphinx3},
	ybar,
	width=\textwidth,
	height=.4\textwidth,
	bar width=.2cm,
	legend style={at={(0.8,1)}, anchor=north,legend columns=-1},
]
\addplot table[x=bench,y=O0]{\suppgccperf};
\addplot table[x=bench,y=O3]{\suppgccperf};
\legend{O0, O3}
\end{axis}
\end{tikzpicture}
\caption{Performance Comparison of Position-Independent O0 and O3 GCC Variants (\%)} \label{fig:suppgcc_perf}
\end{figure}
